# Supplementary material for: Understanding How Network Geometry Influences Diffusion Processes in Complex Networks: A Focus on Cryptocurrency Blockchains and Critical Infrastructure Networks
Source: arXiv:2509.23450 source file (2025-10-09)
Supplement: Supplementary file 1 [file Supplementary_Material.pdf]

# Supporting Information for “Understanding How Network Geometry Influences Diffusion Processes in Complex Networks: A Focus on Cryptocurrency Blockchains and Critical Infrastructure Networks” by S M Mustaquim, Asim K. Dey, and Abhijit Mandal.

## S.1 Additional Results

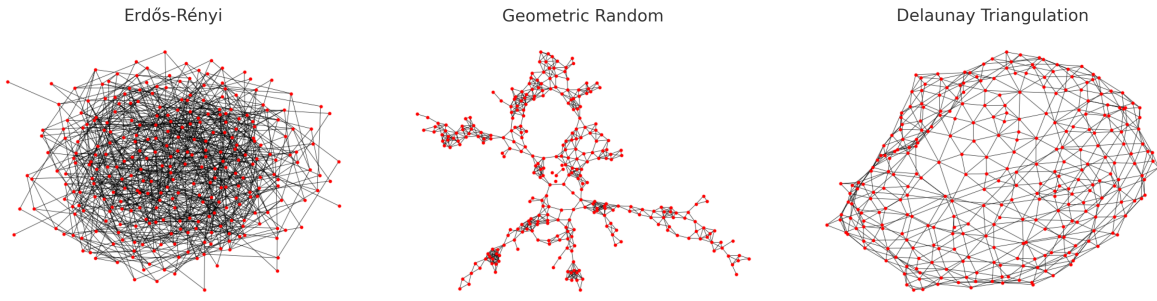

Figure S1: Classical random graph model. (a) ER, (b) GRG, and (c) DT, each with 300 nodes and an expected number of edges of 900.

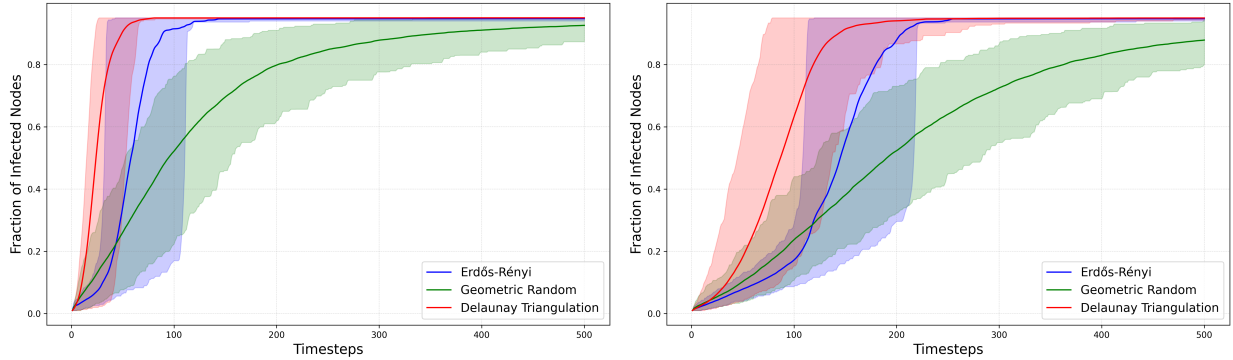

Figure S2: The effect of network structure/topology on the diffusion process. The left panel represents diffusion starting with the top three nodes with the highest betweenness centrality for  $\tau = 0.30$  and the right panel represents the diffusion for  $\tau = 0.40$ , with their corresponding 95% confidence intervals.

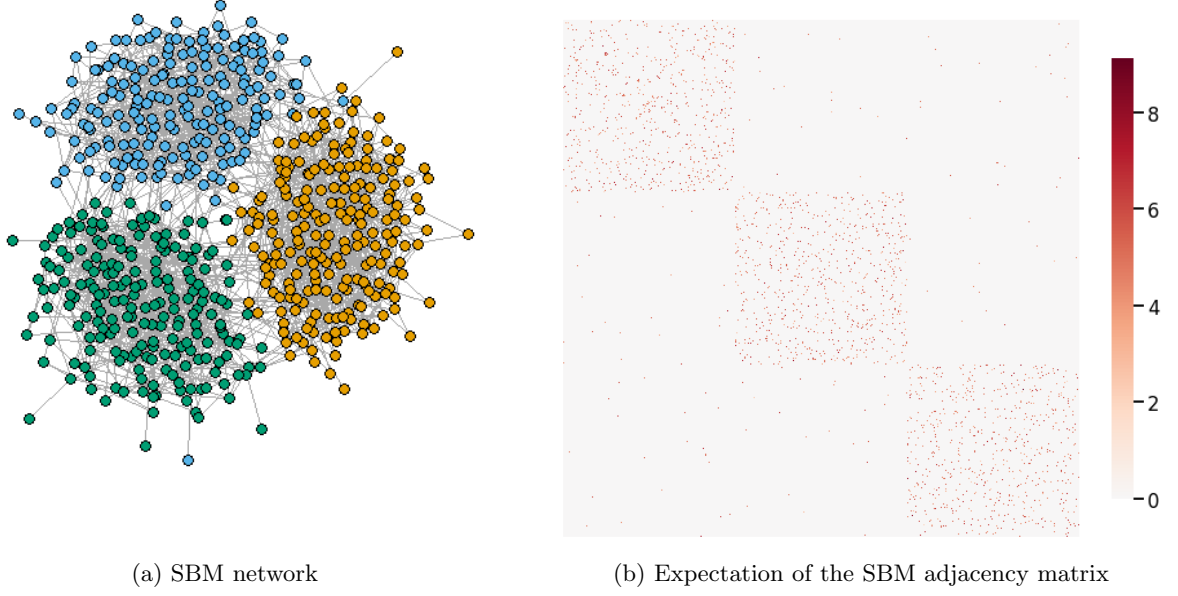

Figure S3: SBM network with parameters  $k = 3$ ,  $p_w = 0.030$  and  $p_b = 0.001$ .

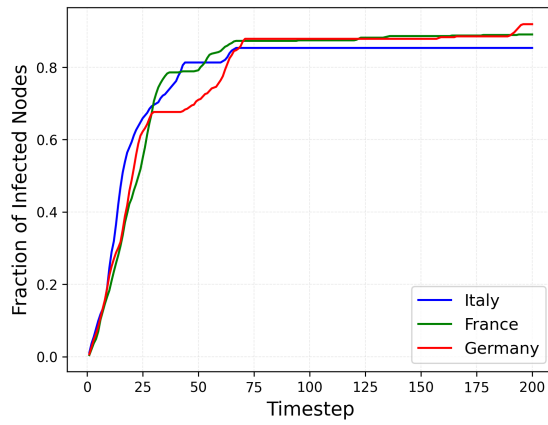

Figure S4: Comparison of fraction of infected nodes over timesteps in 3 European power grid networks, initial infected nodes are selected based on betweenness centrality

## S.2 Diagnostic Plots of Bayesian Inference

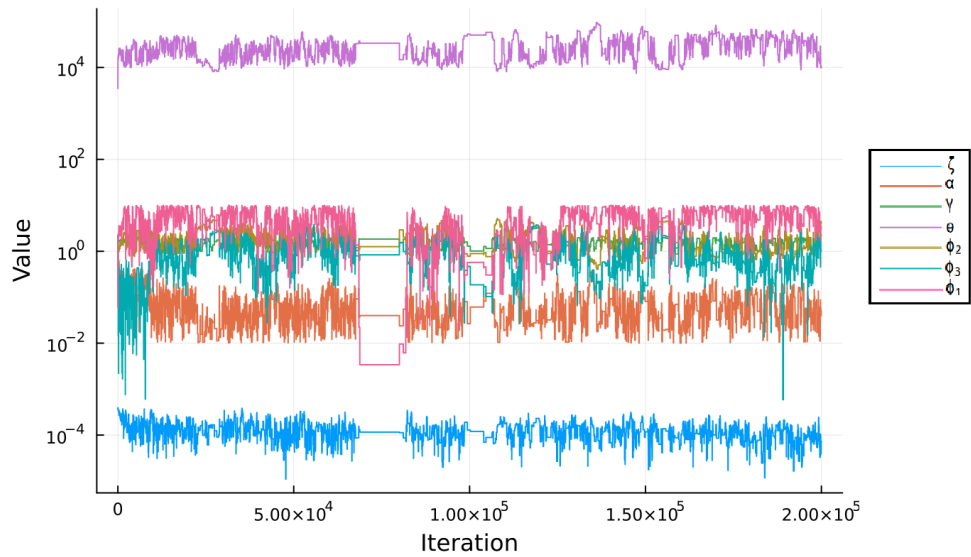

Figure S5: Trace plot of MCMC iterations of Ethereum network.

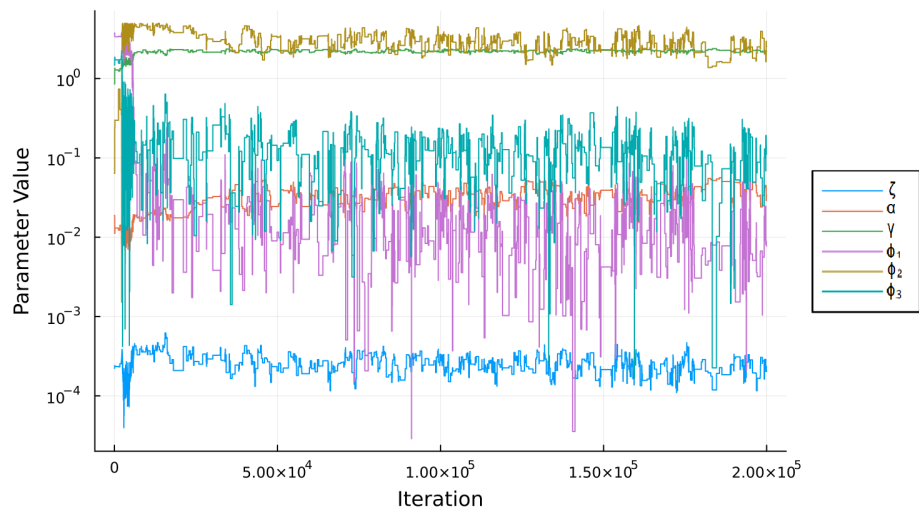

Figure S6: Trace plot of MCMC iterations of the Italian Power grid.

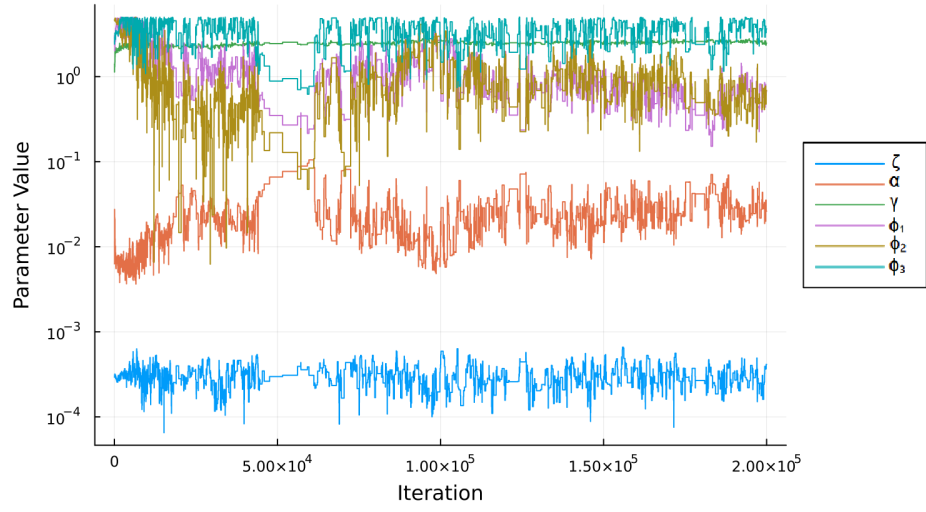

Figure S7: Trace plot of MCMC iterations of the German Power grid.

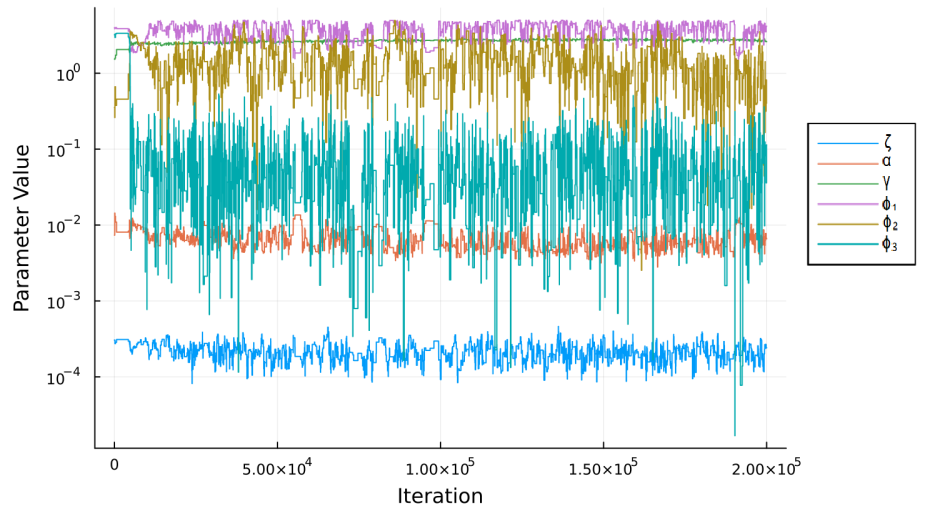

Figure S8: Trace plot of MCMC iterations of the French Power grid.
